# Supplementary material for: A mathematical model for distinguishing bias from sensitivity effects in multialternative detection tasks
Source: arXiv:1310.4219 source file (2013-10-15)
Supplement: Supplementary file 1 [file SI_TablesModel.pdf]

**Table S1. Stimulus-response contingency table for 2-AFC and 2-ADC tasks.**

**A**. 2x2 stimulus-response contingency table for a 2-AFC (Yes/No) task.

| Stimulus \ Response | *Go response @ Loc 1* | *NoGo response* |
|---|---|---|
| *Stimulus @ Loc 1* | Hit (HR) | Miss (MR) |
| *Catch (No stimulus)* | False-alarm (FA) | Correct rejection (CR) |

**B**. 3x3 stimulus-response contingency table for a 2-ADC task.

| Stimulus \ Response | *Go response @ Loc 1* | *Go response @ Loc 2* | *NoGo response* |
|---|---|---|---|
| *Stimulus @ Loc 1* | Hit ($HR_1$) | *False-alarm/ Incorrect response* | Miss ($MR_1$) |
| *Stimulus @ Loc 2* | *False-alarm/ Incorrect response* | Hit ($HR_2$) | Miss ($MR_2$) |
| *Catch (No stimulus)* | False-alarm ($FA_1$) | False-alarm ($FA_2$) | Correct rejection (CR) |

In 2-AFC (Yes/No) tasks there is only one false-alarm: a Go response during catch trials (FA). In addition to this, another type of false-alarm response can occur in 2-ADC tasks: a Go response at a location when a stimulus was presented at the opposite location (gray shaded cells).

**Table S2. Simulated parameter recovery with MLE and MCMC.**

**A.** Parameters used in the simulation.

| Parameter | Location 1 | Location 2 |
|---|---|---|
| *sensitivity* | $d_1 = 1.0$ | $d_2 = 1.0$ |
| *criterion* | $c_1 = -0.25$ | $c_2 = 0.75$ |
| *noise* | $\varepsilon_1 = N(0, 1)$ | $\varepsilon_2 = N(0, 1)$ |
| *stimulus prior probability* | $p_1 = 0.25$ | $p_2 = 0.25$ |

**B.** Simulated contingency table of response counts (N = 4000 trials from 20 simulated runs).

| Stimulus \ Response | *Go response @ Loc 1* | *Go response @ Loc 2* | *NoGo response* |
|---|---|---|---|
| *Stimulus @ Loc 1* | 871 | *66* | 63 |
| *Stimulus @ Loc 2* | *422* | 414 | 164 |
| *Catch (No stimulus)* | 1122 | 263 | 615 |

**C.** Sensitivities and criteria recovered with maximum likelihood (MLE) and Bayesian (Markov Chain Monte Carlo) estimation procedures.

| Parameter | MLE (mean ± SE) | Bayesian (mean ± SE) | 95% CI |
|---|---|---|---|
| *sensitivity* | $d_1 = 1.07 \pm 0.06$ | $d_1 = 1.07 \pm 0.08$ | $d_1$: 0.98 – 1.16 |
| | $d_2 = 0.99 \pm 0.06$ | $d_2 = 0.98 \pm 0.08$ | $d_2$: 0.89 – 1.08 |
| *criterion* | $c_1 = -0.27 \pm 0.03$ | $c_1 = -0.27 \pm 0.03$ | $c_1$: -0.30 – -0.21 |
| | $c_2 = 0.75 \pm 0.04$ | $c_2 = 0.75 \pm 0.05$ | $c_2$: 0.67 – 0.81 |

SE: standard error, CI: credible intervals

**Table S3. Maximum likelihood (ML) estimates of the psychometric function with and without accounting for bias.**

**A.** Parameters used in the simulation of a 2-ADC model with bias ($c_1 \neq c_2$).

| Parameter | | Location 1 | | Location 2 |
|---|---|---|---|---|
| | | $d_{max} = 2.5$ | | $d_{max} = 2.5$ |
| *sensitivity* | $\mathbf{d_1(\xi_1)}$ | $n = 2.0$ | $\mathbf{d_2(\xi_2)}$ | $n = 2.0$ |
| | | $\xi_{50} = 0.35$ | | $\xi_{50} = 0.35$ |
| *criterion* | | $\mathbf{c_1} = 0.1$ | | $\mathbf{c_2} = 0.7$ |
| *noise* | | $\varepsilon_1 = N(0, 1)$ | | $\varepsilon_2 = N(0, 1)$ |
| *stimulus prior probability* | | $p_1 = 0.25$ | | $p_2 = 0.25$ |

**B.** ML estimates of 2-ADC psychometric parameters with and without accounting for bias.

| Parameter | | MLE with bias (mean ± SE) | | MLE without bias (mean ± SE) |
|---|---|---|---|---|
| | | $d_{max} = 2.48 \pm 0.03$ | | $d_{max} = 3.03 \pm 0.05$ |
| | $\mathbf{d_1(\xi_1)}$ | $n = 2.01 \pm 0.05$ | $\mathbf{d_1(\xi_1)}$ | $n = 1.69 \pm 0.04$ |
| | | $\xi_{50} = 0.34 \pm 0.006$ | | $\xi_{50} = 0.33 \pm 0.008$ |
| *sensitivity* | | | | |
| | | $d_{max} = 2.49 \pm 0.03$ | | $d_{max} = 2.49 \pm 0.03$ |
| | $\mathbf{d_2(\xi_2)}$ | $n = 2.03 \pm 0.04$ | $\mathbf{d_2(\xi_2)}$ | $n = 2.95 \pm 0.07$ |
| | | $\xi_{50} = 0.35 \pm 0.005$ | | $\xi_{50} = 0.38 \pm 0.004$ |
| | | $\mathbf{c_1} = 0.10 \pm 0.002$ | | $\mathbf{c_1} = 0.35 \pm 0.002$ |
| *criterion* | | | | |
| | | $\mathbf{c_2} = 0.71 \pm 0.003$ | | $\mathbf{c_2} = 0.35 \pm 0.002$ |
